# Supplementary material for: DynaSLAM II: Tightly-Coupled Multi-Object Tracking and SLAM
Source: arXiv:2010.07820 source file (2020-10-15)
Supplement: Supplementary file 1 [file appendix.tex]

\appendix

The derivative of the term $\Delta \mathbf{T}_{\mathtt{O}_k}^{i,i+1}(\mathbf{w}^k_i, \mathbf{v}^k_i)$ in Eqn.~\ref{eqn: vcte_XYZ} with respect to the angular velocity is approximated as follows. 
Let us apply an additive perturbation $\delta \mathbf{w}^k_i$ to the object angular velocity (Eqn.~\ref{eqn: delta_w}). 
We write only the rotational part of the pose transformation for simplicity.

\begin{equation} \label{eqn: delta_w}
\Delta \mathbf{R}_{\mathtt{O}_k}^{i,i+1} (\mathbf{w}^k_i + \delta \mathbf{w}^k_i) = 
    \text{Exp}((\mathbf{w}^k_i + \delta \mathbf{w}^k_i)\Delta t) 
\end{equation}

We use the first order approximation (Eqn.~\ref{eqn: taylor}), where the term $\mathbf{J}_r$ is the right Jacobian of $\text{SO}(3)$~\cite{forster2016manifold} and
relates additive increments in the tangent space to multiplicative
increments applied on the right-hand side

\begin{equation} \label{eqn: taylor}
\Delta \mathbf{R}_{\mathtt{O}_k}^{i,i+1} (\mathbf{w}^k_i + \delta \mathbf{w}^k_i) \approx
    \text{Exp}(\mathbf{w}^k_i \Delta t) \text{Exp}(\mathbf{J}_r(\mathbf{w}^k_i \Delta t)\delta \mathbf{w}^k_i \Delta t) 
\end{equation}

Assuming that the term $\mathbf{J}_r(\mathbf{w}^k_i \Delta t) \delta \mathbf{w}^k_i \Delta t$ is small, we can rewrite the equation as:

\begin{equation} \label{eqn: Jr_small}
\Delta \mathbf{R}_{\mathtt{O}_k}^{i,i+1} (\mathbf{w}^k_i + \delta \mathbf{w}^k_i) \approx
    \text{Exp}(\mathbf{w}^k_i \Delta t) (\mathbf{I} + [\mathbf{J}_r(\mathbf{w}^k_i \Delta t)\delta \mathbf{w}^k_i \Delta t]_\times),
\end{equation}

where $[\cdot]_\times$ is the skew operator that transforms a vector in $\mathbb{R}3$ into a skew symmetric matrix. 
Therefore, the partial derivative of $\Delta \mathbf{R}_{\mathtt{O}_k}^{i,i+1}$ with respect to the angular velocity can be written as follows:

\begin{equation} \label{eqn: partial}
\frac{\partial \Delta \mathbf{R}_{\mathtt{O}_k}^{i,i+1}}{\partial \delta \mathbf{w}^k_i} = \text{Exp}(\mathbf{w}^k_i \Delta t) [\mathbf{J}_r(\mathbf{w}^k_i \Delta t) \Delta t]_\times
\end{equation}
